# Supplementary material for: DuplexAct: How Interactive Are Frontier Full-Duplex Spoken Language Models?
Source: arXiv:2610.17738 source file (2026-10-13)
Supplement: Supplementary file 1 [file Analysis.tex]

\subsection{Extended Analysis of Direct Replay Performance}
\label{app:direct_replay_analysis}

This analysis expands the immediate-execution comparisons for Wait, Ignore, Take Turn, and Backchannel in Table~\ref{tab:overall_results}. We include the 13 systems with available results and exclude VITA-1.5. BayLing-Duplex is included because its immediate scores are available; its pending subsequent results are not used here. All reported medians are computed across models rather than by pooling trials. Comparisons are descriptive and do not establish statistically significant differences.

\paragraph{Action-level asymmetry.}
The difference between withholding and speech-producing actions is evident both across and within models. Median immediate success is 95.3\% for Wait and 78.8\% for Ignore, versus 30.3\% for Take Turn and 10.8\% for Backchannel. Within 12 of the 13 systems, both Wait and Ignore score higher than either Take Turn or Backchannel. Moshi is the exception, with Take Turn success of 38.0\% exceeding its Ignore score of 32.5\%. Nevertheless, even the highest Take Turn and Backchannel scores remain below 50\%. These results identify condition-appropriate speech production as a shared difficulty within the evaluated Direct Replay tasks, rather than a weakness restricted to a small subset of systems.

\paragraph{Interpreting Take Turn success.}
Take Turn evaluates whether entry occurs within the window required by the interaction condition, covering immediate, delayed, and overlapping entry. A shorter response latency is therefore not uniformly preferable: earlier entry may help an immediate-entry case but violate a delayed-entry requirement. Consequently, the low aggregate scores should not be interpreted simply as evidence that systems respond slowly. They indicate that systems do not reliably meet the entry requirements across the evaluated conditions. However, aggregate scores do not distinguish predominantly early entry, predominantly late entry, absent responses, or condition-specific combinations of these failures. Whether a model follows a relatively fixed timing pattern across conditions must therefore be examined through the condition-level analysis in Section~\ref{sec:condition_analysis}.

\paragraph{Proprietary versus open-source systems.}
Proprietary systems achieve consistently high Wait scores, ranging from 89.5\% to 99.8\%, but do not lead every action. Voila-Autonomous and MiniCPM-o 4.5 share the highest reported Take Turn score of 44.3\%, compared with 41.3\% for Qwen3.5-Omni-Flash-Realtime, the strongest proprietary system on this action. For Backchannel, Raon-SpeechChat reaches 46.2\%, while MiniCPM-o 4.5, Moshi, and BayLing-Duplex also exceed the proprietary maximum of 11.8\%. These comparisons identify strengths of particular open-source models, not a uniform group-level advantage. Indeed, the proprietary group has a higher median Take Turn score than the open-source group, 34.3\% versus 20.2\%. The distinction between the highest-performing individual systems and the broader group distribution is therefore important.

\paragraph{Distinct floor-taking and listener-feedback profiles.}
Raon-SpeechChat exhibits the clearest ranking reversal, combining the highest Backchannel score of 46.2\% with the lowest Take Turn score of 4.3\%. Voila-Autonomous shows the contrasting profile, achieving 44.3\% on Take Turn but only 10.8\% on Backchannel. FLM-Audio similarly achieves 35.2\% on Take Turn but 3.0\% on Backchannel. These differences show that success in taking the floor does not imply comparable success in providing listener feedback. Conversely, MiniCPM-o 4.5 combines the joint-highest Take Turn score with the second-highest Backchannel score of 27.2\%, alongside 95.0\% on Wait and 72.8\% on Ignore. Its broader strengths illustrate that the contrasting profiles of other systems should not be interpreted as evidence that floor-taking and backchannel capabilities are inherently incompatible.

\paragraph{Limits of a restraint--responsiveness interpretation.}
Within the proprietary subset, GPT-Realtime-2.1 and Grok Voice score higher on Wait and Ignore but lower on Take Turn and Backchannel than Gemini 3.1 Flash Live and Qwen3.5-Omni-Flash-Realtime. This is a descriptive pattern within the evaluated subset, rather than evidence of a universal trade-off. Voila-Autonomous combines high Wait and Ignore scores of 96.5\% and 99.2\% with a leading Take Turn score of 44.3\%. Mini-Omni2, by contrast, performs poorly on both withholding and speech-producing actions. Moshi offers another mixed profile, with comparatively strong Take Turn and Backchannel scores of 38.0\% and 22.5\%, but only 32.5\% on Ignore. A single ordering from restrained to responsive therefore does not adequately summarize all observed differences. These cross-model comparisons also do not determine whether changing an individual model's configuration would introduce a trade-off between actions.

\paragraph{Limits of behavioral and architectural interpretation.}
Immediate scores measure satisfaction of action-specific criteria, not the frequency with which a model produces a particular behavior. A low Backchannel score can reflect absent feedback or feedback that fails the required timing or other immediate criteria; it does not by itself establish that a model rarely backchannels. Similarly, successful withholding does not establish deliberate listening, because non-responsiveness can also satisfy a local silence requirement. Section~\ref{sec:subsequent} examines whether successful immediate execution is followed by appropriate continued engagement. Finally, the aggregate profiles do not isolate architectural causes: attributing them to interaction-control mechanisms, training objectives, or decoding strategies requires evidence beyond these action-level scores.


\subsection{Simulator Cue-Landing Coverage}
\label{app:cue_landing}

For \emph{Stop}, \emph{Hold Floor}, and \emph{Recover}, evaluation requires the interaction cue to occur while the model is actively speaking. We therefore record the state in which each injected cue lands: \emph{cue in speaking} indicates that the cue overlaps ongoing model speech; \emph{no response} indicates that the model does not begin speaking after the lead-in; and \emph{cue after finished} indicates that the model responds but finishes before cue injection. Only \emph{cue in speaking} trials enter the headline immediate-execution evaluation for these actions. Table~\ref{tab:simulator_cue_landing} reports the resulting coverage.

\begin{table*}[t]
\centering
\caption{
Cue-landing coverage for simulator-based \emph{Stop}, \emph{Hold Floor}, and \emph{Recover} evaluation. ``Speaking'' denotes cues injected while model speech is ongoing; ``No response'' denotes trials in which the model does not speak after the lead-in; and ``Finished'' denotes trials in which the model finishes speaking before cue injection.
}
\label{tab:simulator_cue_landing}
\scriptsize
\setlength{\tabcolsep}{3.5pt}
\renewcommand{\arraystretch}{1.08}

\begin{tabular}{lrrrrrrrrrrrr}
\toprule
&
\multicolumn{4}{c}{\textbf{Stop}}
&
\multicolumn{4}{c}{\textbf{Hold Floor}}
&
\multicolumn{4}{c}{\textbf{Recover}}
\\
\cmidrule(lr){2-5}
\cmidrule(lr){6-9}
\cmidrule(lr){10-13}

\textbf{Model}
& \textbf{$N$} & \textbf{Speaking} & \textbf{No resp.} & \textbf{Finished}
& \textbf{$N$} & \textbf{Speaking} & \textbf{No resp.} & \textbf{Finished}
& \textbf{$N$} & \textbf{Speaking} & \textbf{No resp.} & \textbf{Finished}
\\
\midrule

GPT-Realtime-2.1
& 200 & 195 & 4 & 1
& 891 & 835 & 54 & 2
& 1200 & 1145 & 52 & 3
\\

Gemini 3.1 Flash Live
& 200 & 195 & 5 & 0
& 891 & 810 & 78 & 3
& 1200 & 1184 & 15 & 1
\\

Qwen3.5-Omni-Flash-Realtime
& 200 & 184 & 13 & 3
& 891 & 717 & 160 & 14
& 1199 & 1107 & 72 & 20
\\

Grok Voice
& 200 & 171 & 20 & 9
& 891 & 642 & 240 & 9
& 1200 & 1118 & 62 & 20
\\

\midrule

Moshi
& 200 & 98 & 42 & 60
& 891 & 571 & 158 & 162
& 1200 & 759 & 278 & 163
\\

FLM-Audio
& 200 & 150 & 48 & 2
& 891 & 545 & 341 & 5
& 1200 & 859 & 332 & 9
\\

BayLing-Duplex
& 199 & 163 & 34 & 2
& 879 & 601 & 261 & 17
& 1198 & 776 & 398 & 24
\\

Raon-SpeechChat
& 200 & 122 & 51 & 27
& 887 & 455 & 344 & 88
& 1200 & 578 & 435 & 187
\\

MiniCPM-o 4.5
& 200 & 170 & 8 & 22
& 891 & 805 & 15 & 71
& 1200 & 1114 & 16 & 70
\\

Freeze-Omni
& 200 & 95 & 101 & 4
& 891 & 442 & 445 & 4
& 1200 & 642 & 555 & 3
\\

\bottomrule
\end{tabular}
\end{table*}
