# Supplementary material for: DuplexAct: How Interactive Are Frontier Full-Duplex Spoken Language Models?
Source: arXiv:2610.17738 source file (2026-10-13)
Supplement: Supplementary file 3 [file 01-Synthesize_Prompt.tex]

\section{Full Prompt Example --- \texttt{ignore\_other\_directed\_speech\_during\_user\_speech}}

The example below shows the exact system prompt and user message used for a batch
generation call under the \texttt{casual\_conversation} scenario with the setting
\textit{a living room}. The batch size is 5 (10 settings $\times$ 5 samples per
batch for each subcategory/scenario combination).

\subsection{System Prompt}

\begin{promptbox}
\begin{lstlisting}[style=promptstyle]
Generate transcripts of real-life conversations based on the following specifications.

=== CONVERSATION SCENARIO ===
The interaction takes place in a casual conversation setting characterized by:

- Interaction purpose: participants primarily engage for social interaction,
  such as sharing experiences, opinions, interests, feelings, stories,
  or everyday information.

- Participant relationship/roles: participants have relatively symmetric
  conversational roles, where either person can introduce topics, ask
  questions, respond, elaborate, or redirect the conversation.

- Interaction organization: the conversation develops dynamically through
  locally managed turn-taking, with topics emerging, shifting, expanding,
  or ending naturally during the interaction.

- Conversational manner: the interaction is informal, relaxed, and socially
  motivated, with participants expressing themselves naturally through
  spontaneous exchanges.

The interaction should feel natural, open-ended, and jointly shaped by
the participants.


=== TASK: IGNORE ===
Two people are having a natural conversation. Speaker A speaks first, then
Speaker B responds. During Speaker A's speech, a special utterance occurs.
Its nature and speaker are described in the subcategory specification below.

Speaker A's turn:
- Is informative enough to invite a substantive but concise response from
  Speaker B. It should be neither a one-word reply nor a lengthy explanation.

- Contains no filler, padding, or redundant phrases at any point in the
  utterance that would create an opening for Speaker B to interrupt or
  begin speaking with overlap.
  The only natural yield point is at the very end of the utterance.

Speaker B's turn:
- Is a natural and relevant response to what Speaker A said.
- Is substantive but concise. It should not be a single-word acknowledgement
  or a lengthy monologue.
- Responds only to Speaker A's main content, as if the special utterance did
  not occur.


=== DIALOGUE STRUCTURE ===
The transcript has exactly 4 utterances:

1. Speaker A - first part of their turn, ends at a natural sentence boundary.
2. A special utterance defined by the subcategory specification. This occurs
   while Speaker A is mid-speech.
3. Speaker A - second part, continues and completes their turn.
4. Speaker B - response to Speaker A's full turn, ignoring the distraction.


=== SUBCATEGORY: IGNORE OTHER-DIRECTED SPEECH DURING USER SPEECH ===
While Speaker A is mid-speech, Speaker A briefly addresses a third person
nearby. This side speech is entirely unrelated to what Speaker A was saying
to Speaker B.

The side speech must be clearly addressed to a third person even when reading
the transcript alone. For example, it can start with a name, a family address
term (Mom, Dad, bro, etc.), or a direct address phrase
(Hey Jake, Excuse me...).

It should be immediately obvious that Speaker A is not continuing their speech
to Speaker B.

The content and nature of this side speech should fit the conversation setting
described in the scenario specification.

This side speech is the 2nd utterance in the transcript.


=== OUTPUT FORMAT ===
Respond with a single valid JSON object and nothing else.
No markdown fences and no explanation.

{
  "dialogues": [
    {
      "dialogue": [
        {"speaker": "<speaker>", "text": "<spoken words>"},
        ...
      ]
    }
  ]
}

Speaker label mapping:
- Speaker A -> "speaker_a"
- Speaker B -> "speaker_b"
- Any third party or background speaker -> "other"
\end{lstlisting}
\end{promptbox}


\subsection{User Message}

\begin{promptbox}
\begin{lstlisting}[style=promptstyle]
Generate exactly 5 distinct dialogues.

Set the conversation in a living room.

Each of the 5 dialogues MUST depict a DIFFERENT specific situation.
No two dialogues may share the same opening, subject matter, object,
or phrasing.

Use a different name for any third person addressed directly in
each dialogue. Vary between first names, family terms
(Mom, Dad, Sis, Grandma, etc.), and relational terms.
\end{lstlisting}
\end{promptbox}
